# Supplementary material for: Split-U-Net: Preventing Data Leakage in Split Learning for Collaborative Multi-Modal Brain Tumor Segmentation
Source: arXiv:2208.10553 source file (2022-09-26)
Supplement: Supplementary file 1 [file suppl.tex]

\subsection{Effect of initialize parameters}
*qualitative segmentation results
Activation maps (dropout, noise) - Batch-size 1
*Robustness analysis of how sensitive the trained model is to the noise inputs.
